# Supplementary material for: QuPeD: Quantized Personalization via Distillation with Applications to Federated Learning
Source: arXiv:2107.13892 source file (2022-07-05)
Supplement: Supplementary file 1 [file appendix_qupel.tex]

For QuPeL, we define the following augmented loss function at client $i$:
\begin{align} 
	F_i(\bx_i,\bc_i,\bw) &:= f_i(\bx_i)+f_i(\widetilde{Q}_{\bc_i}(\bx_i))+\lambda R(\bx_i,\bc_i) + \frac{\lambda_p}{2} (\|\bx_i - \bw \|^2+\|\widetilde{Q}_{\bc_{i}}(\bx_i) - \bw \|^2).  \label{qupel:qupel_problem}
\end{align}
Here, $\bw \in \mathbb{R}^d$ denotes the global model, $\bx_i \in \mathbb{R}^d$ denotes the personalized model at client $i$, and $\bc_i \in \mathbb{R}^{m_i}$ denotes the model quantization centers at client $i$, where $m_i$ is the number of centers at client $i$, with $\log m_i$ representing the number of bits per parameter, which could be different for each client -- larger the $m_i$, higher the precision. Note that different than QuPeD, this time all the model parameters $\bx_i$ are of the same dimension with $\bw$.

From \eqref{qupel:qupel_problem} we get the following global loss function:
\begin{align} 
\arg\min \left(F\big(\{\bx_i\},\{\bc_i\},\bw\big):=\frac{1}{n}\sum_{i=1}^nF_i(\bx_i,\bc_i,\bw) \right),\label{qupel:qupel_global}
\end{align}
where minimization is taken over $\bx_1,\hdots,\bx_n\in\R^d$, $\bc_i\in\R^{m_i}$ for $i\in[n]$, and $\bw\in\R^d$.

We present our proposed algorithm QuPeL for minimizing \eqref{qupel:qupel_global} in Algorithm~\ref{qupel:algo:qupel}.
%As a result we have the following algorithm for optimizing the loss function.
\begin{algorithm}[h]
	\caption{QuPeL}
	{\bf Input:} %Regularization parameters for quantization and personalization  $\lambda,\lambda_p $ respectively, synchronization gap \( \tau \).  For each worker $i$, initial full precision personalized model, initial quantization vectors (centers) and initial local model: $\bz_{i}^{{0}}=(\bx_{i}^{(0)},\bc_{i}^{(0)},\bw_{i}^{(0)})$. A penalty function enforcing quantization $R(\bx,\bc)$, \TODO{a soft quantization function $\widetilde{Q}_{\bc}(\bx)$}. Learning rates $\eta_1,\eta_2,\eta_3$.\\
	Regularization parameters $\lambda,\lambda_p$; synchronization gap $\tau$; for each client $i\in[n]$, initialize full precision personalized model $\bx_i^{0}$, quantization centers $\bc_i^{0}$, and local model $\bw_i^0$; a penalty function enforcing quantization $R(\bx,\bc)$; a soft quantizer $\widetilde{Q}_{\bc}(\bx)$; and learning rates $\eta_1,\eta_2,\eta_3$.\\
	\vspace{-0.3cm}
	\begin{algorithmic}[1] \label{qupel:algo:qupel}
		\FOR{$t=0$ \textbf{to} $T-1$}
		\STATE \textbf{On Clients} $i=1$ \textbf{to} $n$ (in parallel) \textbf{do}:
		\IF{$\tau$ does not divide $t$}
		\STATE Compute $\bg_{i}^{t} := \nabla_{\bx_{i}^{t}} f_i(\bx_{i}^{t}) + \nabla_{\bx_{i}^{t}}f_i(\widetilde{Q}_{\bc_{i}^{t}}(\bx_{i}^{t}))+\lambda_p(\bx_{i}^{t}-\bw_{i}^{t})+ \lambda_p \nabla_{\bx_{i}^{t}}\widetilde{Q}_{\bc_{i}^{t}}(\bx_{i}^{t})(\widetilde{Q}_{\bc_{i}^{t}}(\bx_{i}^{t})-\bw_{i}^{t})  $
		\STATE $\bx_{i}^{t+1}=\text{prox}_{\eta_1 \lambda R_{\bc_{i}^{t}}}(\bx_{i}^{t} - \eta_1 \bg_{i}^{t} )$\\
		\STATE Compute $\bh_i^{t} := \nabla_{\bc_{i}^{t}}  f_i(\widetilde{Q}_{\bc_{i}^{t}}(\bx_{i}^{t+1})) +  \lambda_p \nabla_{\bc_{i}^{t+1}}\widetilde{Q}_{\bc_{i}^{t}}(\bx_{i}^{t+1})(\widetilde{Q}_{\bc_{i}^{t}}(\bx_{i}^{t+1})-\bw_{i}^{t}) $
		\STATE $\bc_{i}^{t+1}=\text{prox}_{\eta_2 \lambda R_{\bx_{i}^{t+1}}}(\bc_{i}^{t}-\eta_2 \bh_i^{t}  )$\\
		\STATE $\bw_{i}^{t+1} = %w_{i,t}-\eta_3 \nabla_{w_{t}} F_i(x_{i,t+1},c_{i,t+1},w_{i,t})=
		\bw_{i}^{t}-\eta_3\lambda_p ((\bw_{i}^{t}-\bx_{i}^{t+1})+ (\bw_{i}^{t}-\widetilde{Q}_{\bc_{i}^{t+1}}(\bx_{i}^{t+1})) $\\
		\ELSE
		\STATE Send $\bw_{i}^{t}$ to \textbf{Server}
		\STATE Receive $\bw^{t}$ from \textbf{Server} and set $\bw_i^{t+1} = \bw^{t}$
		\ENDIF
		\STATE \textbf{On Server do:}
		\IF{$\tau$ divides $t$}
		%		\STATE $\bw^{t+1} = \bw^{t}$
		%		\ELSE
		\STATE Receive $\{\bw_i^{t}\}_{i=1}^n$ and compute $\bw^{t} := \frac{1}{n} \sum_{i=1}^n \bw_i^{t}$
		\STATE Broadcast $\bw^{t}$ to all \textbf{Clients}
		\ENDIF		
		\ENDFOR
		\STATE $\hat{\bx}_{i}^{T} = Q_{\bc_{i}^{T}}(\bx_{i}^{T})$ for all $i \in [n]$
	\end{algorithmic}
	{\bf Output:} Quantized personalized models $\hat{\bx}_i^{T}$ for $i \in [n]$
\end{algorithm}

\subsection{Convergence Analysis}
First we state our convergence result for QuPeL,
\begin{theorem}\label{qupel:thm:personalized}
	Consider running Algorithm \ref{qupel:algo:qupel} $T$ iterations with $\tau \leq \sqrt{T}$, $\eta_1=\frac{1}{2(3\lambda_p+\lambda_pL_{Q_1}+L+GL_{Q_1}+G_{Q_1}Ll_{Q_1})}$, $\eta_2 = \frac{1}{2(\lambda_p+\lambda_pL_{Q_2}+GL_{Q_2}+G_{Q_2}LL_{Q_2})}$, and $\eta_3 = \nicefrac{1}{8\lambda_p\sqrt{T}}$.
	For any $t\in[T]$, define $\bG_{i}^{t} := [\nabla_{\bx_{i}^{t+1}} F_i(\bx_{i}^{t+1},\bc_{i}^{t},\bw^{t})^T, \\ \nabla_{\bc_{i}^{t+1}} F_i(\bx_{i}^{t+1},\bc_{i}^{t+1},\bw^{t})^T, \nabla_{\bw^{t}} F_i(\bx_{i}^{t+1},\bc_{i}^{t+1},\bw^{t})^T]^T$.
	%$\bG_{i}^{t}:=[\bG_{i,1}^t\ \bG_{i,2}^t\ \bG_{i,3}^t]^T$, where $\bG_{i,1}^t=\nabla_{\bx_{i}^{t+1}} F_i(\bx_{i}^{t+1},\bc_{i}^{t},\bw^{t})^T$, $\bG_{i,2}^t=\nabla_{\bc_{i}^{t+1}} F_i(\bx_{i}^{t+1},\bc_{i}^{t+1},\bw^{t})^T$, $\bG_{i,3}^t=\nabla_{\bw^{t}} F_i(\bx_{i}^{t+1},\bc_{i}^{t+1},\bw^{t})^T$.
	Then, under assumptions {\bf A.1-A.6}, we have:
	%
	%	\begin{align*}
	%	\frac{1}{T}\sum_{t=0}^{T-1}\frac{1}{n}\sum_{i=1}^{n} \Big\|G_{i,t}\Big\|^2 \leq& \frac{54(L^{(i)}_{max})^2\tau\kappa+108(L^{(i)}_{max})^2+288(L^{(i)}_{max})^2\lambda_p \Delta_F}{\sqrt{T}} + \frac{189\tau^2\kappa+\frac{3}{4}\tau^2\kappa^2}{T} + \frac{378\tau^2\kappa}{T^{\frac{3}{2}}}+ 216\kappa
	%	\end{align*}
	\begin{align*}
		\frac{1}{T}\sum_{t=0}^{T-1}\frac{1}{n}\sum_{i=1}^{n} \Big\|\bG_{i}^{t}\Big\|^2 &= \mathcal{O} \left( \frac{\Lambda}{\sqrt{T}} + \frac{L_{\max}^2\tau^2\kappa+\tau^2\kappa^2}{T}+\frac{L_{\max}^2\tau^2\kappa}{T^{\frac{3}{2}}}+ L_{\max}^2\kappa \right) ,
	\end{align*}
	where $L_{\max} = \max\{\sqrt{\frac{1}{18}},\frac{2\lambda_p}{3}+\frac{2\lambda_pL_{Q_2}}{3}+ GL_{Q_2}+G_{Q_2}LL_{Q_2},\frac{7}{3}\lambda_p+\frac{2\lambda_pL_{Q_1}}{3}+\frac{\lambda_pG_{Q_1}l_{Q_1}}{3}+ L+Gl_{Q_1}+G_{Q_1}Ll_{Q_1}\}$, and $\Lambda = L_{\max}^2\tau\kappa(1+G^2_{Q_1}+G^2_{Q_2})+L_{\max}^2+L_{\max}^2\lambda_p \Delta_F$ with $\Delta_F=\frac{1}{n}\sum_{i=1}^{n}\left(F_i(\bx_{i}^{0},\bc_{i}^{0},\bw_{i}^{0})-F_i(\bx_{i}^{T},\bc_{i}^{T},\bw_{i}^{T})\right)$. %$L_{max} =\max\{\lambda_p+L+GL_{Q_2}+G_{Q_2}Ll_{Q_2},GL_{Q_1}+G_{Q_1}Ll_{Q_1},1\}$, and $\kappa=\frac{1}{n}\sum_{i=1}^n \kappa_i$.
\end{theorem}
The rest of this section is devoted to proving Theorem~\ref{qupel:thm:personalized}.

The analysis is similar to the one in Appendix~\ref{appendix:proof of theorem 2}, however, this time we can assume same gradient bounds for each client since all the clients have the same model structure. As a result the analysis requires slightly less algebraic manipulations. Naturally, we don't need \textbf{A.7} in this analysis. We defer proofs of the claims and some derivation details to the end of section. We take $\bw^t = \frac{1}{n}\sum_{i=1}^n \bw^t_{i}$, so that $\bw^t$ is defined for every time point.

\textbf{Alternating updates.} Let us first restate the alternating updates for $\bx_i$ and $\bc_i$:
\begin{align*}
	\bx^{t+1}_{i} &= \text{prox}_{\eta_1 \lambda R_{\bc^t_{i}}}(\bx^t_{i}-\eta_1 \nabla f_i(\bx^t_{i})- \eta_1 \nabla_{\bx^t_{i}} f_i(\widetilde{Q}_{\bc^t_{i}}(\bx^t_{i}))-\eta_1 \lambda_p(\bx^t_{i}-\bw^{t}_{i}) \\
	& \quad  + \nabla_{\bx_{i}^{t}}\widetilde{Q}_{\bc_{i}^{t}}(\bx_{i}^{t})(\widetilde{Q}_{\bc_{i}^{t}}(\bx_{i}^{t})-\bw_{i}^{t}) )\\
	\bc^{t+1}_{i} &= \text{prox}_{\eta_2 \lambda R_{\bx^{t+1}_{i}}}(\bc^t_{i}-\eta_2 \nabla_{\bc^t_{i}} f_i(\widetilde{Q}_{\bc^t_{i}}(\bx^t_{i})) -\eta_2\lambda_p \nabla_{\bc_{i}^{t+1}}\widetilde{Q}_{\bc_{i}^{t}}(\bx_{i}^{t+1})(\widetilde{Q}_{\bc_{i}^{t}}(\bx_{i}^{t+1})-\bw_{i}^{t}))
\end{align*}
The alternating updates are equivalent to solving the following two optimization problems.
\begin{align}
	\bx^{t+1}_{i}&= \underset{\bx \in \mathbb{R}^{d}}{\arg \min }\left\{\left\langle \bx-\bx^t_{i}, \nabla f_i\left(\bx^t_{i}\right)\right\rangle+\left\langle \bx-\bx^t_{i}, \nabla_{\bx^t_{i}} f_i(\widetilde{Q}_{\bc^t_{i}}(\bx^t_{i}))\right\rangle +\left\langle \bx-\bx^t_{i}, \lambda_p (\bx^t_{i}-\bw^{t}_{i})\right\rangle \right. \notag \\
	&\hspace{2cm} \left. +\left\langle \bx-\bx^t_{i}, \lambda_p \nabla_{\bx_{i}^{t}}\widetilde{Q}_{\bc_{i}^{t}}(\bx_{i}^{t})(\widetilde{Q}_{\bc_{i}^{t}}(\bx_{i}^{t})-\bw_{i}^{t}) \right\rangle + \frac{1}{2 \eta_1}\left\|\bx-\bx^t_{i}\right\|_{2}^{2}+\lambda R(\bx,\bc^t_{i})\right\} \label{qupel:thm2:lower-bounding-interim1}\\
	\bc^{t+1}_{i}&= \underset{\bc \in \mathbb{R}^{m}}{\arg \min }\left\{\left\langle \bc-\bc^t_{i}, \nabla_{\bc^t_{i}} f_i(\widetilde{Q}_{\bc^t_{i}}(\bx^{t+1}_{i}))\right\rangle + \left\langle \bc-\bc^t_{i}, \lambda_p \nabla_{\bc_{i}^{t+1}}\widetilde{Q}_{\bc_{i}^{t}}(\bx_{i}^{t+1})(\widetilde{Q}_{\bc_{i}^{t}}(\bx_{i}^{t+1})-\bw_{i}^{t}) \right\rangle \right. \notag \\
	& \hspace{2cm} \left.  +\frac{1}{2 \eta_2}\left\|\bc-\bc^t_{i}\right\|_{2}^{2}+\lambda R(\bx^{t+1}_{i},\bc)\right\} \label{qupel:thm2:lower-bounding-interim2}
\end{align}
%Let us state some useful facts.
%\begin{fact}
Note that the update on $\bw^t$ from Algorithm~\ref{qupel:algo:qupel} can be written as:
\begin{align*}
	\bw^{t+1} = \bw^{t} - \eta_3 \bg^{t}, \quad \text{ where }\quad \bg^{t} =\frac{1}{n} \sum_{i=1}^n \nabla_{\bw^{t}_{i}} F_i(\bx^{t+1}_{i},\bc^{t+1}_{i},\bw^{t}_{i}).
	%	\bw^{t+1} = \bw^{t} - \eta_3 \frac{1}{n} \sum_{i=1}^n \nabla_{\bw^{t}_{i}} F_i(\bx^{t+1}_{i},\bc^{t+1}_{i},\bw^{t}_{i})
\end{align*}
%\end{fact}
%We will denote $\bg^{t} =\frac{1}{n} \sum_{i=1}^n \nabla_{\bw^{t}_{i}} F_i(\bx^{t+1}_{i},\bc^{t+1}_{i},\bw^{t}_{i})$. Then $\bw^{t+1} = \bw^{t} - \eta_3 \bg^{t}$.
In the convergence analysis we will require smoothness of the local functions $F_i$ w.r.t.\ the global parameter $\bw$. Recall the definition of $F_i(\bx_i,\bc_i,\bw) = f_i(\bx_i)+f_i(\widetilde{Q}_{\bc_i}(\bx_i))+\lambda R(\bx_i,\bc_i) + \frac{\lambda_p}{2} (\|\bx_i - \bw \|^2+\|\widetilde{Q}_{\bc_{i}}(\bx_i) - \bw \|^2)$ from \eqref{qupel:qupel_problem}. It follows that $F_i$ is $2\lambda_p$-smooth with respect to $\bw$:
%\begin{fact}\label{qupel:thm2:lambda_p}
%Recall the definition of $F_i(\bx,\bc,\bw)$ from \eqref{qpfl} in Section~\ref{sec:problem}. Then, $F_i$ is $\lambda_p$-smooth with respect to $\bw$:
\begin{align}\label{qupel:lambda_p}
	\Big\| \nabla_\bw F_i(\bx,\bc,\bw)-\nabla_{\bw'} F_i(\bx,\bc,\bw')\Big\| &=\|\lambda_p(2\bw-\bx-\widetilde{Q}_{\bc}(\bx))-\lambda_p(2\bw'-\bx-\widetilde{Q}_{\bc}(\bx))\| \notag \\ &\leq 2\lambda_p \|\bw-\bw'\|, \quad \forall \bw,\bw' \in \mathbb{R}^d.
\end{align}
%\end{fact}
Now let us move on with the proof. %First we will show the sufficient decrease properties.
\subsection{Sufficient Decrease} \label{qupel:thm2:subsection sufficient decrease}
We will divide this part into three and obtain sufficient decrease properties for each variable: $\bx_i,\bc_i,\bw$.
\subsubsection{Sufficient Decrease Due to $\bx_i$}
We begin with a useful claim.
\begin{claim} \label{qupel:thm2:claim lqxsmoothness}
	$f_i(\bx)+ f_i(\widetilde{Q}_\bc(\bx))+\frac{\lambda_p}{2}(\|\bx-\bw\|^2+\|\widetilde{Q}_{\bc}(\bx)-\bw\|^2)$ is $(\lambda_p+\lambda_pL_{Q_1}+L+GL_{Q_1}+G_{Q_1}Ll_{Q_1})$-smooth with respect to $\bx$.
\end{claim}
From Claim~\ref{qupel:thm2:claim lqxsmoothness} we have:

\begin{align}
	&F_i(\bx^{t+1}_{i},\bc^t_{i},\bw^{t}) +(\frac{1}{2\eta_1}-\frac{\lambda_p+\lambda_pL_{Q_1}+L+GL_{Q_1}+G_{Q_1}Ll_{Q_1}}{2})\|\bx^{t+1}_{i}-\bx^t_{i}\|^2 \notag \\
	& \quad = f_i(\bx^{t+1}_{i})+f_i(\widetilde{Q}_{\bc^t_{i}}(\bx^{t+1}_{i})) +\lambda R(\bx^{t+1}_{i},\bc^t_{i}) + \frac{\lambda_p}{2}\|\bx^{t+1}_{i}-\bw^{t}\|^2 \notag \\
	& \hspace{1cm}+ \frac{\lambda_p}{2}\|\widetilde{Q}_{\bc^t_{i}}(\bx^{t+1}_{i})-\bw^{t}\|^2  + (\frac{1}{2\eta_1}-\frac{\lambda_p+\lambda_pL_{Q_1}+L+GL_{Q_1}+G_{Q_1}Ll_{Q_1}}{2})\|\bx^{t+1}_{i}-\bx^t_{i}\|^2 \notag \\ 
	&\quad\leq f_i(\bx^t_{i})+f_i(\widetilde{Q}_{\bc^t_{i}}(\bx^t_{i}))+\frac{\lambda_p}{2}\|\bx^t_{i}-\bw^{t}\|^2+ \frac{\lambda_p}{2}\|\widetilde{Q}_{\bc^t_{i}}(\bx^{t}_{i})-\bw^{t}\|^2 +\lambda R(\bx^{t+1}_{i},\bc^t_{i}) \notag \\ 
	&\hspace{1cm} +\left\langle \nabla f_i(\bx^t_{i}), \bx^{t+1}_{i}-\bx^t_{i}\right\rangle + \left\langle \nabla_{\bx^t_{i}} f_i(\widetilde{Q}_{\bc^t_{i}}(\bx^t_{i})), \bx^{t+1}_{i}-\bx^t_{i}\right\rangle+\left\langle \lambda_p(\bx^t_{i}-\bw^{t}_{i}), \bx^{t+1}_{i}-\bx^t_{i}\right\rangle \notag \\
	&\hspace{1cm}  + \left\langle \lambda_p \nabla_{\bx_{i}^{t}}\widetilde{Q}_{\bc_{i}^{t}}(\bx_{i}^{t})(\widetilde{Q}_{\bc_{i}^{t}}(\bx_{i}^{t})-\bw_{i}^{t}), \bx^{t+1}_{i}-\bx^t_{i}\right\rangle +  \left\langle \lambda_p(\bw^{t}_{i}-\bw^{t}), \bx^{t+1}_{i}-\bx^t_{i}\right\rangle \notag \\
	& \hspace{1cm}+ \left\langle \lambda_p\nabla_{\bx_{i}^{t}}\widetilde{Q}_{\bc_{i}^{t}}(\bx_i^t)(\bw^{t}_{i}-\bw^{t}), \bx^{t+1}_{i}-\bx^t_{i}\right\rangle + \frac{1}{2\eta_1}\|\bx^{t+1}_{i}-\bx^t_{i}\|^2 \label{qupel:thm2:first-part-interim1}
\end{align}
\begin{claim}\label{qupel:thm2:claim:lower-bound1}
	Let 
	\begin{align*}
		A(\bx^{t+1}_{i}) &:= \lambda R(\bx^{t+1}_{i},\bc^t_{i})+\left\langle \nabla f_i(\bx^t_{i}), \bx^{t+1}_{i}-\bx^t_{i}\right\rangle 
		+ \left\langle \nabla_{\bx^t_{i}} f_i(\widetilde{Q}_{\bc^t_{i}}(\bx^t_{i})), \bx^{t+1}_{i}-\bx^t_{i}\right\rangle \notag \\
		&\hspace{1cm}+ \left\langle \lambda_p \nabla_{\bx_{i}^{t}}\widetilde{Q}_{\bc_{i}^{t}}(\bx_{i}^{t})(\widetilde{Q}_{\bc_{i}^{t}}(\bx_{i}^{t})-\bw_{i}^{t}), \bx^{t+1}_{i}-\bx^t_{i}\right\rangle +\left\langle \lambda_p(\bx^t_{i}-\bw^{t}_{i}), \bx^{t+1}_{i}-\bx^t_{i}\right\rangle \notag \\
		& \hspace{1 cm} + \frac{1}{2\eta_1}\|\bx^{t+1}_{i}-\bx^t_{i}\|^2 \notag \\
		A(\bx^t_{i}) &:= \lambda R(\bx^t_{i},\bc^t_{i}).
	\end{align*} 
	Then $A(\bx^{t+1}_{i})\leq A(\bx^t_{i})$.
	%\begin{align}
	%&\lambda R(\bx^{t+1}_{i},\bc^t_{i})+\left\langle \nabla f_i(\bx^t_{i}), \bx^{t+1}_{i}-\bx^t_{i}\right\rangle 
	%+ \left\langle \nabla_x f_i(\widetilde{Q}_{\bc^t_{i}}(\bx^t_{i})), \bx^{t+1}_{i}-\bx^t_{i}\right\rangle \notag \\
	%&\hspace{3cm} +\left\langle \lambda_p(\bx^t_{i}-\bw^{t}_{i}), \bx^{t+1}_{i}-\bx^t_{i}\right\rangle + \frac{1}{2\eta_1}\|\bx^{t+1}_{i}-\bx^t_{i}\|^2 \leq \lambda R(\bx^t_{i},\bc^t_{i})
	%\end{align}
\end{claim}
Using the inequality from Claim~\ref{qupel:thm2:claim:lower-bound1} in \eqref{qupel:thm2:first-part-interim1} gives
\begin{align}
	F_i(\bx^{t+1}_{i},\bc^t_{i},\bw^{t})\ +\ &(\frac{1}{2\eta_1}-\frac{\lambda_p+\lambda_p L_{Q_1}+L+GL_{Q_1}+G_{Q_1}Ll_{Q_1}}{2})\|\bx^{t+1}_{i}-\bx^t_{i}\|^2 \notag \\
	&\stackrel{\text{(a)}}{\leq} f_i(\bx^t_{i})+f_i(\widetilde{Q}_{\bc^t_{i}}(\bx^t_{i}))+\frac{\lambda_p}{2}\|\bx^t_{i}-\bw^{t}\|^2+\frac{\lambda_p}{2}\|\widetilde{Q}_{\bc^t_{i}}(\bx^t_{i})-\bw^{t}\|^2 + A(\bx^{t+1}_{i}) \notag \\
	& \quad + \left\langle \lambda_p\nabla_{\bx_{i}^{t}}\widetilde{Q}_{\bc_{i}^{t}}(\bx_i^t)(\bw^{t}_{i}-\bw^{t}), \bx^{t+1}_{i}-\bx^t_{i}\right\rangle + \left\langle\lambda_p(\bw^{t}_{i}-\bw^{t}), \bx^{t+1}_{i}-\bx^t_{i}\right\rangle \notag \\
	&\stackrel{\text{(b)}}{\leq} f_i(\bx^t_{i})+f_i(\widetilde{Q}_{\bc^t_{i}}(\bx^t_{i}))+\frac{\lambda_p}{2}\|\bx^t_{i}-\bw^{t}\|^2 +\frac{\lambda_p}{2}\|\widetilde{Q}_{\bc^t_{i}}(\bx^t_{i})-\bw^{t}\|^2 + \lambda R(\bx^t_{i},\bc^t_{i}) \notag \\
	& \quad +\frac{\lambda_p(1+G^2_{Q_1})}{2}\|\bw^{t}_{i}-\bw^{t}\|^2  +  \lambda_p\|\bx^{t+1}_{i}-\bx^t_{i}\|^2 \notag \\
	&= F_i(\bx^t_{i},\bc^t_{i},\bw^{t}) + \frac{\lambda_p(1+G^2_{Q_1})}{2}\|\bw^{t}_{i}-\bw^{t}\|^2+\lambda_p\|\bx^{t+1}_{i}-\bx^t_{i}\|^2 \label{qupel:thm2:first-part-interim3}
\end{align}
To obtain (a), we substituted the value of $A(\bx^{t+1}_{i})$ from Claim~\ref{qupel:thm2:claim:lower-bound1} into \eqref{qupel:thm2:first-part-interim1}. In (b), we used $A(\bx^{t+1}_{i})\leq \lambda R(\bx^t_{i},\bc^t_{i})$ and $\langle\lambda_p(\bw^{t}_{i}-\bw^{t}), \bx^{t+1}_{i}-\bx^t_{i}\rangle = \langle\sqrt{\lambda_p}(\bw^{t}_{i}-\bw^{t}), \sqrt{\lambda_p}(\bx^{t+1}_{i}-\bx^t_{i})\rangle \leq \frac{\lambda_p}{2}\|\bw^{t}_{i}-\bw^{t}\|^2 + \frac{\lambda_p}{2}\|\bx^{t+1}_{i}-\bx^t_{i}\|^2$, and 
\begin{align*}
\left\langle \lambda_p\nabla_{\bx_{i}^{t}}\widetilde{Q}_{\bc_{i}^{t}}(\bx_i^t)(\bw^{t}_{i}-\bw^{t}), \bx^{t+1}_{i}-\bx^t_{i}\right\rangle &\leq \frac{\lambda_p}{2}\left\|\widetilde{Q}_{\bc_{i}^{t}}(\bx_i^t)(\bw^{t}_{i}-\bw^{t})\right\|_2^2 + \frac{\lambda_p}{2}\|\bx^{t+1}_{i}-\bx^t_{i}\|^2 \notag \\
&\leq \frac{\lambda_p}{2}\left\|\widetilde{Q}_{\bc_{i}^{t}}(\bx_i^t)\right\|_F^2\|\bw^{t}_{i}-\bw^{t}\|_2^2 + \frac{\lambda_p}{2}\|\bx^{t+1}_{i}-\bx^t_{i}\|^2 \notag \\
&\leq \frac{\lambda_pG^2_{Q_1}}{2}\|\bw^{t}_{i}-\bw^{t}\|^2 + \frac{\lambda_p}{2}\|\bx^{t+1}_{i}-\bx^t_{i}\|^2,
\end{align*}
where the second inequality follows from $\|A\bx\|_2\leq\|A\|_F\|\bx\|_2$, which holds for any matrix $A$ and vector $\bx$ (dimension compatible); and the third inequality uses Assumption {\bf A.5}.

Substituting $\eta_1=\frac{1}{2(3\lambda_p+\lambda_pL_{Q_1}+L+GL_{Q_1}+G_{Q_1}Ll_{Q_1})}$ in \eqref{qupel:thm2:first-part-interim3} gives:

\begin{align} \label{qupel:thm2:dec1}
	F_i(\bx^{t+1}_{i},\bc^t_{i},\bw^{t})
	+(\frac{3\lambda_p+\lambda_pL_{Q_1}+L+GL_{Q_1}+G_{Q_1}Ll_{Q_1}}{2})\|\bx^{t+1}_{i}-\bx^t_{i}\|^2 &\leq F_i(\bx^t_{i},\bc^t_{i},\bw^{t}) \notag \\
	& \hspace{-2cm} +\frac{\lambda_p(1+G^2_{Q_1})}{2}\|\bw^{t}_{i}-\bw^{t}\|^2
\end{align}
\subsubsection{Sufficient Decrease Due to $\bc_i$}
In parallel with Claim~\ref{qupel:thm2:claim lqxsmoothness}, we have following smoothness result for $\bc$:
\begin{claim} \label{qupel:thm2:claim lqcsmoothness}
	$f_i(\widetilde{Q}_\bc(\bx)) + \frac{\lambda_p}{2}(\|\widetilde{Q}_{\bc}(\bx)-\bw\|^2)$ is $(\lambda_pL_{Q_2}+GL_{Q_2}+G_{Q_2}Ll_{Q_2})$-smooth with respect to $\bc$.
\end{claim}
From Claim \ref{qupel:thm2:claim lqcsmoothness} we have:
\begin{align}
	&F_i(\bx^{t+1}_{i},\bc^{t+1}_{i},\bw^{t})+(\frac{1}{2\eta_2}-\frac{\lambda_pL_{Q_2}+GL_{Q_2}+G_{Q_2}Ll_{Q_2}}{2})\|\bc^{t+1}_{i}-\bc^t_{i}\|^2 \notag \\
	& \hspace{1cm}= f_i(\bx^{t+1}_{i})+f_i(\widetilde{Q}_{\bc^{t+1}_{i}}(\bx^{t+1}_{i}))+\lambda R(\bx^{t+1}_{i},\bc^{t+1}_{i})+ \frac{\lambda_p}{2}\|\widetilde{Q}_{\bc^t_{i}}(\bx^{t+1}_{i})-\bw^{t}\|^2 \notag \\
	&\hspace{2cm}+\frac{\lambda_p}{2}\|\bx^{t+1}_{i}-\bw^{t}\|^2 + (\frac{1}{2\eta_2}-\frac{\lambda_pL_{Q_2}+GL_{Q_2}+G_{Q_2}Ll_{Q_2}}{2})\|\bc^{t+1}_{i}-\bc^t_{i}\|^2 \notag \\ 
	&\hspace{1cm}\leq f_i(\bx^{t+1}_{i})+f_i(\widetilde{Q}_{\bc^t_{i}}(\bx^{t+1}_{i}))+\lambda R(\bx^{t+1}_{i},\bc^{t+1}_{i})+\frac{\lambda_p}{2}\|\widetilde{Q}_{\bc^t_{i}}(\bx^{t+1}_{i})-\bw^{t}\|^2 \notag \\
	&\hspace{2cm} +\frac{\lambda_p}{2}\|\bx^{t+1}_{i}-\bw^{t}\|^2+ \left\langle \nabla_{\bc^t_{i}} f_i(\widetilde{Q}_{\bc^t_{i}}(\bx^{t+1}_{i})), \bc^{t+1}_{i}-\bc^t_{i}\right\rangle + \frac{1}{2\eta_2}\|\bc^{t+1}_{i}-\bc^t_{i}\|^2 \notag  \\
	& \hspace{2cm} + \left\langle \lambda_p \nabla_{\bc_{i}^{t}}\widetilde{Q}_{\bc_{i}^{t}}(\bx_{i}^{t+1})(\widetilde{Q}_{\bc_{i}^{t}}(\bx_{i}^{t+1})-\bw_{i}^{t}), \bc^{t+1}_{i}-\bc^t_{i}\right\rangle \\
	& \hspace{2cm }+ \left\langle \lambda_p \nabla_{\bc_{i}^{t}}\widetilde{Q}_{\bc_{i}^{t}}(\bx_{i}^{t+1})(\bw_i^{t}-\bw^{t}), \bc^{t+1}_{i}-\bc^t_{i}\right\rangle \label{qupel:thm2:second-part-interim1}
\end{align}

\begin{claim} \label{qupel:thm2:claim:lower-bound2}
	Let 
	\begin{align*}
		B(\bc^{t+1}_{i}) &:= \lambda R(\bx^{t+1}_{i},\bc^{t+1}_{i}) + \left\langle \nabla_{\bc^t_{i}} f_i(\widetilde{Q}_{\bc^t_{i}}(\bx^{t+1}_{i})), \bc^{t+1}_{i}-\bc^t_{i}\right\rangle \notag  + \frac{1}{2\eta_2}\|\bc^{t+1}_{i}-\bc^t_{i}\|^2 \notag \\
		& \quad + \left\langle \lambda_p  \nabla_{\bc_{i}^{t+1}}\widetilde{Q}_{\bc_{i}^{t}}(\bx_{i}^{t+1})(\widetilde{Q}_{\bc_{i}^{t}}(\bx_{i}^{t+1})-\bw_{i}^{t}), \bc^{t+1}_{i}-\bc^t_{i}\right\rangle \\
		B(\bc^t_{i}) &:= \lambda R(\bx^{t+1}_{i},\bc^t_{i}).
	\end{align*} 
	Then $B(\bc^{t+1}_{i})\leq B(\bc^t_{i})$.
\end{claim}
Substituting the bound from Claim~\ref{qupel:thm2:claim:lower-bound2} in \eqref{qupel:thm2:second-part-interim1}, 

\begin{align*}
	& F_i(\bx^{t+1}_{i},\bc^{t+1}_{i},\bw^{t})+(\frac{1}{2\eta_2}-\frac{\lambda_pL_{Q_2}+GL_{Q_2}+G_{Q_2}LL_{Q_2}}{2})\|\bc^{t+1}_{i}-\bc^t_{i}\|^2 \\
	& \hspace{1cm} \leq f_i(\bx^{t+1}_{i})+f_i(\widetilde{Q}_{\bc^t_{i}}(\bx^{t+1}_{i}))+\lambda R(\bx^{t+1}_{i},\bc^t_{i}) +\frac{\lambda_p}{2}\|\bx^{t+1}_{i}-\bw^{t}\|^2 \\
	& \hspace{2cm} +\frac{\lambda_p}{2}\|\widetilde{Q}_{\bc^t_{i}}(\bx^{t+1}_{i})-\bw^{t}\|^2+ \left\langle \lambda_p \nabla_{\bc_{i}^{t}}\widetilde{Q}_{\bc_{i}^{t}}(\bx_{i}^{t+1})(\bw_i^{t}-\bw^{t}), \bc^{t+1}_{i}-\bc^t_{i}\right\rangle \\
	& \hspace{1cm} = F_i(\bx^{t+1}_i,\bc^{t}_i,\bw^t) + \frac{\lambda_p}{2}\|\bc^{t+1}_{i}-\bc^t_{i}\|^2 + \frac{\lambda_p G^{2}_{Q_2}}{2}\|\bw_i^{t}-\bw^{t}\|^2
\end{align*}

Substituting $\eta_2 = \frac{1}{2(\lambda_p+\lambda_pL_{Q_2}+GL_{Q_2}+G_{Q_2}LL_{Q_2})}$ gives us: 
\begin{align} \label{qupel:thm2:dec2}
	F_i(\bx^{t+1}_{i},\bc^{t+1}_{i},\bw^{t})+\frac{\lambda_p+\lambda_pL_{Q_2}+GL_{Q_2}+G_{Q_2}LL_{Q_2}}{2}\|\bc^{t+1}_{i}-\bc^t_{i}\|^2  &\leq	F_i(\bx^{t+1}_{i},\bc^t_{i},\bw^{t}) \notag \\
	& + \frac{\lambda_p G^{2}_{Q_2}}{2}\|\bw_i^{t}-\bw^{t}\|^2.
\end{align}

\subsubsection{Sufficient Decrease Due to $\bw$}
Now, we use $2\lambda_p$-smoothness of $F_i(\bx,\bc,\bw)$ with respect to $\bw$:
\begin{align*}
	F_i(\bx^{t+1}_{i},\bc^{t+1}_{i},\bw^{t+1}) &\leq 	F_i(\bx^{t+1}_{i},\bc^{t+1}_{i},\bw^{t}) + \left\langle \nabla_{\bw^{t}} F_i(\bx^{t+1}_{i},\bc^{t+1}_{i},\bw^{t}), \bw^{t+1}-\bw^{t} \right\rangle \\
	& \quad+ \lambda_p\|\bw^{t+1}-\bw^{t}\|^2 
\end{align*}
Then we have,
\begin{align*}
	F_i(\bx^{t+1}_{i},\bc^{t+1}_{i},\bw^{t+1}) &\leq 	F_i(\bx^{t+1}_{i},\bc^{t+1}_{i},\bw^{t}) + \left\langle \nabla_{\bw^{t}} F_i(\bx^{t+1}_{i},\bc^{t+1}_{i},\bw^{t}), \bw^{t+1}-\bw^{t} \right\rangle \\
	& \quad + \lambda_p\|\bw^{t+1}-\bw^{t}\|^2 \\
	&= F_i(\bx^{t+1}_{i},\bc^{t+1}_{i},\bw^{t}) + \left\langle \nabla_{\bw^{t}} F_i(\bx^{t+1}_{i},\bc^{t+1}_{i},\bw^{t}), \eta_3 \bg^{t} \right\rangle + \lambda_p\|\eta_3 \bg^{t}\|^2 \\
	& =	F_i(\bx^{t+1}_{i},\bc^{t+1}_{i},\bw^{t}) -  \eta_3 \left\langle \nabla_{\bw^{t}} F_i(\bx^{t+1}_{i},\bc^{t+1}_{i},\bw^{t}), \bg^{t} - \nabla_{\bw^{t}} F_i(\bx^{t+1}_{i},\bc^{t+1}_{i},\bw^{t}) \right. \\
	& \left. \quad + \nabla_{\bw^{t}} F_i(\bx^{t+1}_{i},\bc^{t+1}_{i},\bw^{t}) \right\rangle  \\
	& \quad + \lambda_p{2}\eta_3^2\|\bg^{t} - \nabla_{\bw^{t}} F_i(\bx^{t+1}_{i},\bc^{t+1}_{i},\bw^{t}) + \nabla_{\bw^{t}} F_i(\bx^{t+1}_{i},\bc^{t+1}_{i},\bw^{t})\|^2 \\ 
	&=	F_i(\bx^{t+1}_{i},\bc^{t+1}_{i},\bw^{t}) - \eta_3\Big\|\nabla_{\bw^{t}} F_i(\bx^{t+1}_{i},\bc^{t+1}_{i},\bw^{t})\Big\|^2 \\& \quad -  \eta_3 \left\langle \nabla_{\bw^{t}} F_i(\bx^{t+1}_{i},\bc^{t+1}_{i},\bw^{t}), \bg^{t} - \nabla_{\bw^{t}} F_i(\bx^{t+1}_{i},\bc^{t+1}_{i},\bw^{t}) \right\rangle  \\& \quad + \lambda_p\eta_3^2\|\bg^{t} - \nabla_{\bw^{t}} F_i(\bx^{t+1}_{i},\bc^{t+1}_{i},\bw^{t}) + \nabla_{\bw^{t}} F_i(\bx^{t+1}_{i},\bc^{t+1}_{i},\bw^{t})\|^2 \\ 
	& \leq F_i(\bx^{t+1}_{i},\bc^{t+1}_{i},\bw^{t}) - \eta_3\Big\|\nabla_{\bw^{t}} F_i(\bx^{t+1}_{i},\bc^{t+1}_{i},\bw^{t})\Big\|^2 \\
	& \quad + \frac{\eta_3}{2}\Big\|\nabla_{\bw^{t}} F_i(\bx^{t+1}_{i},\bc^{t+1}_{i},\bw^{t})\Big\|^2  + \frac{\eta_3}{2}\Big\|\bg^{t} - \nabla_{\bw^{t}} F_i(\bx^{t+1}_{i},\bc^{t+1}_{i},\bw^{t})\Big\|^2\\
	& \quad + 2\lambda_p \eta_3^2 \left( \Big\|\bg^{t} - \nabla_{\bw^{t}} F_i(\bx^{t+1}_{i},\bc^{t+1}_{i},\bw^{t})\Big\|^2 + \Big\|\nabla_{\bw^{t}} F_i(\bx^{t+1}_{i},\bc^{t+1}_{i},\bw^{t})\Big\|^2 \right)
	\\ & = F_i(\bx^{t+1}_{i},\bc^{t+1}_{i},\bw^{t}) - (\frac{\eta_3}{2}-2\lambda_p\eta_3^2)\Big\|\nabla_{\bw^{t}} F_i(\bx^{t+1}_{i},\bc^{t+1}_{i},\bw^{t})\Big\|^2 \\& \quad + (\frac{\eta_3}{2}+2\lambda_p\eta_3^2)\Big\|\bg^{t} - \nabla_{\bw^{t}_{i}} F_i(\bx^{t+1}_{i},\bc^{t+1}_{i},\bw^{t}_{i}) + \nabla_{\bw^{t}_{i}} F_i(\bx^{t+1}_{i},\bc^{t+1}_{i},\bw^{t}_{i}) \\ & \quad - \nabla_{\bw^{t}} F_i(\bx^{t+1}_{i},\bc^{t+1}_{i},\bw^{t})\Big\|^2  \\
	& \leq F_i(\bx^{t+1}_{i},\bc^{t+1}_{i},\bw^{t}) - (\frac{\eta_3}{2}-2\lambda_p\eta_3^2)\Big\|\nabla_{\bw^{t}} F_i(\bx^{t+1}_{i},\bc^{t+1}_{i},\bw^{t})\Big\|^2 \\
	`& \quad + (\eta_3+4\lambda_p\eta_3^2)\Big\|\bg^{t} - \nabla_{\bw^{t}_{i}} F_i(\bx^{t+1}_{i},\bc^{t+1}_{i},\bw^{t}_{i})\Big\|^2 \\
	& \quad + (\eta_3+4\lambda_p\eta_3^2)\Big\|\nabla_{\bw^{t}_{i}} F_i(\bx^{t+1}_{i},\bc^{t+1}_{i},\bw^{t}_{i}) - \nabla_{\bw^{t}} F_i(\bx^{t+1}_{i},\bc^{t+1}_{i},\bw^{t})\Big\|^2 \\
	& \leq F_i(\bx^{t+1}_{i},\bc^{t+1}_{i},\bw^{t}) - (\frac{\eta_3}{2}-2\lambda_p\eta_3^2)\Big\|\nabla_{\bw^{t}} F_i(\bx^{t+1}_{i},\bc^{t+1}_{i},\bw^{t})\Big\|^2 \\& \quad + (\eta_3+4\lambda_p\eta_3^2)\Big\|\bg^{t} - \nabla_{\bw^{t}_{i}} F_i(\bx^{t+1}_{i},\bc^{t+1}_{i},\bw^{t}_{i})\Big\|^2 \\
	& \quad + (\eta_3+4\lambda_p\eta_3^2)4\lambda_p^2\Big\|\bw^{t}_{i}-\bw^{t}\Big\|^2
\end{align*}

Rearranging the terms, we have:
\begin{align} \label{qupel:thm2:dec3}
	&F_i(\bx^{t+1}_{i},\bc^{t+1}_{i},\bw^{t+1}) \notag + (\frac{\eta_3}{2}-2\lambda_p\eta_3^2)\Big\|\nabla_{\bw^{t}} F_i(\bx^{t+1}_{i},\bc^{t+1}_{i},\bw^{t})\Big\|^2  \\
	& \hspace{1cm} \leq (\eta_3+4\lambda_p\eta_3^2)\Big\|\bg^{t} - \nabla_{\bw^{t}_{i}} F_i(\bx^{t+1}_{i},\bc^{t+1}_{i},\bw^{t}_{i})\Big\|^2 \notag + (\eta_3+4\lambda_p\eta_3^2)4\lambda_p^2\Big\|\bw^{t}_{i}-\bw^{t}\Big\|^2 \notag \\
	& \hspace{2cm}+ F_i(\bx^{t+1}_{i},\bc^{t+1}_{i},\bw^{t}) 
\end{align}

\subsubsection{Overall Decrease} 
Define 
\begin{align}
L_{x} &= 3\lambda_p+\lambda_pL_{Q_1}+L+GL_{Q_1}+G_{Q_1}Ll_{Q_1} \label{qupel_L_x-defn} \\
L_{c} &= \lambda_p+\lambda_pL_{Q_2}+GL_{Q_2}+G_{Q_2}Ll_{Q_2}. \label{qupel_L_c-defn} 
\end{align}
Summing \eqref{qupel:thm2:dec1}, \eqref{qupel:thm2:dec2}, \eqref{qupel:thm2:dec3} we get the overall decrease property:

\begin{align} \label{qupel:thm2:dec4}
	&F_i(\bx^{t+1}_{i},\bc^{t+1}_{i},\bw^{t+1}) + (\frac{\eta_3}{2}-2\lambda_p\eta_3^2)\Big\|\nabla_{\bw^{t}} F_i(\bx^{t+1}_{i},\bc^{t+1}_{i},\bw^{t})\Big\|^2 \ + \frac{L_{x}}{2}\|\bx^{t+1}_{i}-\bx^t_{i}\|^2 \notag \\
	& \quad + \frac{L_{c}}{2}\|\bc^{t+1}_{i}-\bc^t_{i}\|^2 \leq   (\eta_3+4\lambda_p\eta_3^2)\Big\|\bg^{t} - \nabla_{\bw^{t}_{i}} F_i(\bx^{t+1}_{i},\bc^{t+1}_{i},\bw^{t}_{i})\Big\|^2 \notag \\
	& \hspace{1cm} + (1+G^2_{Q_1}+G^2_{Q_2}+4\eta_3\lambda_p+16\lambda_p^2\eta_3^2)\lambda_p\|\bw^{t}_{i}-\bw^{t}\|^2 + F_i(\bx^t_{i},\bc^t_{i},\bw^{t})  
\end{align}
Let 
\begin{align}
L_{\min} = \min\{L_{x},L_{c},(\eta_3-4\lambda_p\eta_3^2)\}. \label{qupel_L_min-defn}
\end{align}
Then,
\begin{align} \label{qupel:thm2:dec5}
	&F_i(\bx^{t+1}_{i},\bc^{t+1}_{i},\bw^{t+1}) + \frac{L_{\min}}{2}\left(\Big\|\nabla_{\bw^{t}} F_i(\bx^{t+1}_{i},\bc^{t+1}_{i},\bw^{t})\Big\|^2 \ +\|\bx^{t+1}_{i}-\bx^t_{i}\|^2 +\|\bc^{t+1}_{i}-\bc^t_{i}\|^2\right) \notag \\
	&\leq (\eta_3+4\lambda_p\eta_3^2)\Big\|\bg^{t} - \nabla_{\bw^{t}_{i}} F_i(\bx^{t+1}_{i},\bc^{t+1}_{i},\bw^{t}_{i})\Big\|^2 +  F_i(\bx^t_{i},\bc^t_{i},\bw^{t}) \notag \\
	& \hspace{2cm} + (1+G^2_{Q_1}+G^2_{Q_2}+4\eta_3\lambda_p+16\lambda_p^2\eta_3^2)\lambda_p\|\bw^{t}_{i}-\bw^{t}\|^2
\end{align}
\subsection{Bound on the Gradient}
Now, we will use the first order optimality conditions due to proximal updates and bound the partial gradients with respect to variables $\bx$ and $\bc$. After obtaining bounds for partial gradients we will bound the overall gradient and use our results from Section~\ref{qupel:thm2:subsection sufficient decrease} to arrive at the final bound.

\subsubsection{Bound on the Gradient w.r.t.\ $\bx_i$}
Taking the derivative inside the minimization problem \eqref{qupel:thm2:lower-bounding-interim1} with respect to $\bx$ at $\bx=\bx^{t+1}_{i}$ and setting it to $0$ gives the following optimality condition:

\begin{align}
	\nabla f_i(\bx^t_{i})+\nabla_{\bx^t_{i}} f_i(\widetilde{Q}_{\bc^t_{i}}(\bx^t_{i})) + \lambda_p(\bx^t_{i}-\bw^{t}_{i}) &+ \lambda_p\nabla_{\bx^t_{i}} \widetilde{Q}_{\bc^t_{i}}(\bx^t_{i}) (\widetilde{Q}_{\bc^t_{i}}(\bx^t_{i})-\bw^{t}_{i}) \notag \\
	&+\frac{1}{\eta_1}(\bx^{t+1}_{i}-\bx^t_{i})+\lambda\nabla_{\bx^{t+1}_{i}} R(\bx^{t+1}_{i},\bc^t_{i}) = 0  \label{qupel:thm3-popt11}
\end{align}

Then we have,
\begin{align*}
	\Big\|\nabla_{\bx^{t+1}_{i}} F_i(\bx^{t+1}_{i},\bc^t_{i},\bw^{t})\Big\| &= \Big\|\nabla f_i(\bx^{t+1}_{i}) + \nabla_{\bx^{t+1}_{i}} f_i(\widetilde{Q}_{\bc^t_{i}}(\bx^{t+1}_{i})) + \lambda_p(\bx^{t+1}_{i}-\bw^{t}) \\
	& \quad+ \lambda_p\nabla_{\bx^{t+1}_{i}} \widetilde{Q}_{\bc^t_{i}}(\bx^{t+1}_{i}) (\widetilde{Q}_{\bc^t_{i}}(\bx^{t+1}_{i})-\bw^{t}) + \lambda \nabla_{\bx^{t+1}_{i}} R(\bx^{t+1}_{i},\bc^t_{i})\Big\| \\
	&\stackrel{\text{(a)}}{=} \Big\|\nabla f_i(\bx^{t+1}_{i})-\nabla f_i(\bx^t_{i}) + \nabla_{\bx^{t+1}_{i}} f_i(\widetilde{Q}_{\bc^t_{i}}(\bx^{t+1}_{i}))-\nabla_{\bx^t_{i}} f_i(\widetilde{Q}_{\bc^t_{i}}(\bx^t_{i}))\\
	& \quad + \lambda_p\nabla_{\bx^{t+1}_{i}} \widetilde{Q}_{\bc^t_{i}}(\bx^{t+1}_{i}) (\widetilde{Q}_{\bc^t_{i}}(\bx^{t+1}_{i})-\bw^{t}) \\
	& \quad - \lambda_p\nabla_{\bx^{t}_{i}} \widetilde{Q}_{\bc^t_{i}}(\bx^{t}_{i}) (\widetilde{Q}_{\bc^t_{i}}(\bx^{t}_{i})-\bw^{t}_i)\\
	& \quad +(\lambda_p-\frac{1}{\eta_1})(\bx^{t+1}_{i}-\bx^t_{i}) + \lambda_p(\bw^{t}_{i}-\bw^{t})\Big\| \\
	& \leq (\frac{1}{\eta_1} + \lambda_p+\lambda_pG_{Q_1}l_{Q_1}+L+GL_{Q_1}+G_{Q_1}Ll_{Q_1})\|\bx^{t+1}_{i}-\bx^t_{i}\| \\
	& \quad +\lambda_p(1+G_{Q_1})\|\bw^{t}_{i}-\bw^{t}\|\\
\end{align*}
where (a) is from \eqref{qupel:thm3-popt11} and the last inequality is due to Lipschitz continuous gradients and triangle inequality. This implies: \\
\begin{align*}
	\Big\|\nabla_{\bx^{t+1}_{i}} F_i(\bx^{t+1}_{i},\bc^t_{i},\bw^{t})\Big\|^2 &\leq 2(\frac{1}{\eta_1} + \lambda_p+\lambda_pG_{Q_1}l_{Q_1}+L+GL_{Q_1}+G_{Q_1}Ll_{Q_1})^2\|\bx^{t+1}_{i}-\bx^t_{i}\|^2 \\  & \quad +2\lambda_p^2(1+G_{Q_1})^2\|\bw^{t}_{i}-\bw^{t}\|^2
\end{align*}
Substituting $\eta_1=\frac{1}{2(3\lambda_p+\lambda_pL_{Q_1}+L+GL_{Q_1}+G_{Q_1}Ll_{Q_1})}$ we have:
\begin{align} \label{qupel:thm2:partial grad1}
	\Big\|\nabla_{\bx^{t+1}_{i}} F_i(\bx^{t+1}_{i},\bc^t_{i},\bw^{t})\Big\|^2 &\leq 2(7\lambda_p+2\lambda_pL_{Q_1}+\lambda_pG_{Q_1}l_{Q_1}\notag\\
	& \quad +3(L+GL_{Q_1}+G_{Q_1}Ll_{Q_1}))^2\|\bx^{t+1}_{i}-\bx^t_{i}\|^2 \notag \\
	& \quad +2\lambda_p^2(1+G_{Q_1})^2\|\bw^{t}_{i}-\bw^{t}\|^2 \notag \\
	& = 18(\frac{7}{3}\lambda_p+\frac{2\lambda_pL_{Q_1}}{3}+\frac{\lambda_pG_{Q_1}l_{Q_1}}{3}+ L+Gl_{Q_1}\notag\\
	& \quad +G_{Q_1}Ll_{Q_1})^2\|\bx^{t+1}_{i}-\bx^t_{i}\|^2 \notag \\
	& \quad +2\lambda_p^2(1+G_{Q_1})^2\|\bw^{t}_{i}-\bw^{t}\|^2
\end{align}
\subsubsection{Bound on the Gradient w.r.t.\ $\bc_i$}
Similarly. taking the derivative inside the minimization problem \eqref{qupel:thm2:lower-bounding-interim2} with respect to $\bc$ at $\bc^{t+1}_{i}$ and setting it to $0$ gives the following optimality condition:
\begin{align}
	&\nabla_{\bc^t_{i}} f_i(\widetilde{Q}_{\bc^t_{i}}(\bx^{t+1}_{i})) +\frac{1}{\eta_2}(\bc^{t+1}_{i}-\bc^t_{i}) +\lambda_p\nabla_{\bc^t_{i}} \widetilde{Q}_{\bc^t_{i}}(\bx^{t+1}_{i}) (\widetilde{Q}_{\bc^t_{i}}(\bx^{t+1}_{i})-\bw^{t}_{i}) \notag \\
	& \hspace{7cm}+\lambda\nabla_{\bc^{t+1}_{i}} R(\bx^{t+1}_{i},\bc^{t+1}_{i}) = 0 \label{qupel:thm3-popt21}
\end{align}
Then we have 
\begin{align*}
	\Big\|\nabla_{\bc^{t+1}_{i}} F_i(\bx^{t+1}_{i},\bc^{t+1}_{i},\bw^{t})\Big\| &= \Big\| \nabla_{\bc^{t+1}_{i}} f_i(\widetilde{Q}_{\bc^{t+1}_{i}}(\bx^{t+1}_{i})) + \lambda_p\nabla_{\bc^{t+1}_{i}} \widetilde{Q}_{\bc^{t+1}_{i}}(\bx^{t+1}_{i}) (\widetilde{Q}_{\bc^{t+1}_{i}}(\bx^{t+1}_{i})-\bw^{t}_{i}) \\
	& \hspace{2cm} + \lambda \nabla_{\bc^{t+1}_{i}} R(\bx^{t+1}_{i},\bc^{t+1}_{i})\Big\|
	\\ &= \Big\| \nabla_{\bc^{t+1}_{i}} f_i(\widetilde{Q}_{\bc^{t+1}_{i}}(\bx^{t+1}_{i})) - \nabla_{\bc^t_{i}} f_i(\widetilde{Q}_{\bc^t_{i}}(\bx^{t+1}_{i})) + \frac{1}{\eta_2}(\bc^t_{i}-\bc^{t+1}_{i})\\
	& \quad +\lambda_p\nabla_{\bc^{t+1}_{i}} \widetilde{Q}_{\bc^{t+1}_{i}}(\bx^{t+1}_{i}) (\widetilde{Q}_{\bc^{t+1}_{i}}(\bx^{t+1}_{i}) - \bw_i^t) \\ 
	& \quad -  \lambda_p\nabla_{\bc^{t}_{i}} \widetilde{Q}_{\bc^{t}_{i}}(\bx^{t+1}_{i}) (\widetilde{Q}_{\bc^{t}_{i}}(\bx^{t+1}_{i})-\bw^t)\Big\|\\
	& \leq (\frac{1}{\eta_2}+ \lambda_pG_{Q_2}l_{Q_2}+GL_{Q_2}+G_{Q_2}Ll_{Q_2})\|\bc^{t+1}_{i}-\bc^t_{i}\| \\
	& \quad + \lambda_pG_{Q_2}\|\bw_i^t-\bw^t\|\\
\end{align*}

the first equality is due to \eqref{qupel:thm3-popt21} and the last inequality is due to Lipschitz continuous gradient and triangle inequality. As a result we have, 
\begin{align} \label{qupel:thm2:partial grad2}
	\Big\|\nabla_{\bc^{t+1}_{i}} F_i(\bx^{t+1}_{i},\bc^{t+1}_{i},\bw^{t})\Big\|^2 &\leq 2(\frac{1}{\eta_2}+ \lambda_pG_{Q_2}l_{Q_2}+GL_{Q_2}+G_{Q_2}Ll_{Q_2})^2\|\bc^{t+1}_{i}-\bc^t_{i}\|^2 \notag \\
	& \hspace{2cm} + 2\lambda_p^2G^2_{Q_2}\|\bw_i^t-\bw^t\|^2
\end{align}

substituting $\eta_2 = \frac{1}{2(\lambda_p+\lambda_pL_{Q_2}+GL_{Q_2}+G_{Q_2}LL_{Q_2})}$ we have:
\begin{align*}
	\Big\|\nabla_{\bc^{t+1}_{i}} F_i(\bx^{t+1}_{i},\bc^{t+1}_{i},\bw^{t})\Big\|^2 &\leq 18( \frac{2\lambda_p}{3}+\frac{2\lambda_pL_{Q_2}}{3}+ GL_{Q_2}+G_{Q_2}LL_{Q_2})^2\|\bc^{t+1}_{i}-\bc^t_{i}\|^2 \\
	& \hspace{2cm} + 2\lambda_p^2G^2_{Q_2}\|\bw_i^t-\bw^t\|^2
\end{align*}
\subsubsection{Overall Bound}
Then, let us write $\|\bG^{t}_{i}\|^2:$
\begin{align*}
	\|\bG^{t}_{i}\|^2 & = \Big\|[\nabla_{\bx^{t+1}_{i}} F_i(\bx^{t+1}_{i},\bc^t_{i},\bw^{t})^T,\nabla_{\bc^{t+1}_{i}} F_i(\bx^{t+1}_{i},\bc^{t+1}_{i},\bw^{t})^T , \nabla_{\bw^{t}} F_i(\bx^{t+1}_{i},\bc^{t+1}_{i},\bw^{t})^T]^T\Big\|^2 \\
	& = \Big\|\nabla_{\bx^{t+1}_{i}} F_i(\bx^{t+1}_{i},\bc^t_{i},\bw^{t})\Big\|^2 + \Big\|\nabla_{\bc^{t+1}_{i}} F_i(\bx^{t+1}_{i},\bc^{t+1}_{i},\bw^{t})\Big\|^2 + \Big\|\nabla_{\bw^{t}} F_i(\bx^{t+1}_{i},\bc^{t+1}_{i},\bw^{t})\Big\|^2 \\
	& \leq 18(\frac{7}{3}\lambda_p+\frac{2\lambda_pL_{Q_1}}{3}+\frac{\lambda_pG_{Q_1}l_{Q_1}}{3}+ L+Gl_{Q_1}+G_{Q_1}Ll_{Q_1})^2\|\bx^{t+1}_{i}-\bx^t_{i}\|^2  \\ 
	&\quad + 18( \frac{2\lambda_p}{3}+\frac{2\lambda_pL_{Q_2}}{3}+ GL_{Q_2}+G_{Q_2}LL_{Q_2})^2\|\bc^{t+1}_{i}-\bc^t_{i}\|^2 +\Big\| \nabla_{\bw^{t}} F_i(\bx^{t+1}_{i},\bc^{t+1}_{i},\bw^{t})\Big\|^2 \\
	& \quad +2\lambda_p^2((1+G_{Q_1})^2+G^2_{Q_2})\|\bw^{t}_{i}-\bw^{t}\|^2
\end{align*}

where the last inequality is due to \eqref{qupel:thm2:partial grad1} and \eqref{qupel:thm2:partial grad2}. Let 
\begin{align}
L_{\max} &= \max\left\{\sqrt{\frac{1}{18}},\frac{2\lambda_p}{3}+\frac{2\lambda_pL_{Q_2}}{3}+ GL_{Q_2}+G_{Q_2}LL_{Q_2}, \right. \notag \\
&\left.\hspace{3cm} \frac{7}{3}\lambda_p+\frac{2\lambda_pL_{Q_1}}{3}+\frac{\lambda_pG_{Q_1}l_{Q_1}}{3}+ L+Gl_{Q_1}+G_{Q_1}Ll_{Q_1}\right\}. \label{qupel_L_max-defn}
\end{align}
Then,
\begin{align} \label{qupel:thm2:bound over gradient}
	&\Big\|[\nabla_{\bx^{t+1}_{i}} F_i(\bx^{t+1}_{i},\bc^t_{i},\bw^{t})^T,\nabla_{\bc^{t+1}_{i}} F_i(\bx^{t+1}_{i},\bc^{t+1}_{i},\bw^{t})^T , \nabla_{\bw^{t}} F_i(\bx^{t+1}_{i},\bc^{t+1}_{i},\bw^{t})^T]^T\Big\|^2 \notag\\
	& \leq 18L_{\max}^2(\|\bx^{t+1}_{i}-\bx^t_{i}\|^2+\|\bc^{t+1}_{i}-\bc^t_{i}\|^2+\Big\|\nabla_{\bw^{t}} F_i(\bx^{t+1}_{i},\bc^{t+1}_{i},\bw^{t})\Big\|^2) \notag \\
	& \hspace{2cm} +2\lambda_p^2((1+G_{Q_1})^2+G^2_{Q_2})\|\bw^{t}_{i}-\bw^{t}\|^2 \notag\\
	&\stackrel{\text{(a)}}{\leq}  36\frac{L_{\max}^2}{L_{\min}} \Big[(\eta_3+4\lambda_p\eta_3^2)\Big\|\bg^{t} - \nabla_{\bw^{t}_{i}} F_i(\bx^{t+1}_{i},\bc^{t+1}_{i},\bw^{t}_{i})\Big\|^2 \notag \\ 
	& \hspace{1cm}+ (1+G^2_{Q_1}+G^2_{Q_2}+4\eta_3\lambda_p+16\lambda_p^2\eta_3^2)\lambda_p\|\bw^{t}_{i}-\bw^{t}\|^2 \notag\\ 
	& \hspace{1cm}  + F_i(\bx^t_{i},\bc^t_{i},\bw^{t}) - F_i(\bx^{t+1}_{i},\bc^{t+1}_{i},\bw^{t+1}) \Big]+2\lambda_p^2((1+G_{Q_1})^2+G^2_{Q_2})\|\bw^{t}_{i}-\bw^{t}\|^2. 
\end{align}
In (a) we use the bound from \eqref{qupel:thm2:dec5}, and $L_{\min}$ is defined in \eqref{qupel_L_min-defn}. 

Now we state a useful lemma that enables us to relate local version of the global model, $\bw_i$, to global model itself, $\bw$.
\begin{lemma}\label{qupel:thm2:lemma1}
	Let $\eta_3$ be chosen such that $\eta_3 \leq \sqrt{\frac{1}{48\tau^2\lambda_p^2}}$, then we have,
	\begin{align*} 
		\frac{1}{T}\sum_{t=0}^{T-1}\frac{1}{n}\sum_{i=1}^{n} \|\bw^{t}-\bw^{t}_{i}\|^2 \leq 6 \tau^2\eta_3^2\kappa. 
	\end{align*}
\end{lemma}
As a corollary:
\begin{corollary}\label{qupel:thm2:corollary diversity}
	Recall, $\bg^{t} = \frac{1}{n} \sum_{i=1}^n \nabla_{\bw^{t}} F_i(\bx^{t+1}_{i},\bc^{t+1}_{i},\bw^{t}_{i})$. Then, we have:
	\begin{align*}
		\frac{1}{T}\sum_{t=0}^{T-1} \frac{1}{n} \sum_{i=1}^n \Big\|\bg^{t} - \nabla_{\bw^{t}_{i}} F_i(\bx^{t+1}_{i},\bc^{t+1}_{i},\bw^{t}_{i})\Big\|^2 \leq 144\lambda_p^2\tau^2\eta_3^2\kappa+3\kappa.
	\end{align*}
\end{corollary}
See end of the section for the proofs. Using Lemma~\ref{qupel:thm2:lemma1} and Corollary~\ref{qupel:thm2:corollary diversity}, summing the bound in \eqref{qupel:thm2:bound over gradient} over time and clients, dividing by $T$ and $n$:
%1/(12L^lam2sqrtT)
\begin{align} \label{qupel:thm2:res1}
	\nonumber \frac{1}{T}\sum_{t=0}^{T-1}\frac{1}{n}\sum_{i=1}^{n} \|\bG^{t}_{i}\|^2 &\leq 36\frac{L_{\max}^2}{L_{\min}} \Big[(\eta_3+4\lambda_p\eta_3^2)(144\lambda_p^2\tau^2\eta_3^2\kappa+3\kappa) \notag  \\
	& \hspace{1cm}+(1+G^2_{Q_1}+G^2_{Q_2}+4\eta_3\lambda_p+16\lambda_p^2\eta_3^2)\lambda_p6\tau^2\eta_3^2\kappa \nonumber \\
	& \hspace{1cm} +\frac{\sum_{i=1}^{n}\left(F_i(\bx^{0}_{i},\bc^{0}_{i},\bw^{0}_{i})-F_i(\bx^T_{i},\bc^T_{i},\bw^{T}_{i})\right)}{nT}\Big] \notag \\
	& \hspace{1cm} + 2\lambda_p^2((1+G_{Q_1})^2+G^2_{Q_2})6\tau^2\eta_3^2\kappa \notag  \\
	& = 36\frac{L_{\max}^2}{L_{\min}} \Big[6\tau^2\eta_3^2\kappa(\lambda_p(1+G^2_{Q_1}+G^2_{Q_2})+28\eta_3\lambda_p^2+112\eta_3^2\lambda_p^3) \notag \\
	& \hspace{1cm}+3\eta_3\kappa+12\lambda_p\eta_3^2\kappa+ \frac{\Delta_F}{T}\Big] + 12\lambda_p^2((1+G_{Q_1})^2+G^2_{Q_2})\tau^2\eta_3^2\kappa
\end{align}

where $\Delta_F=\frac{\sum_{i=1}^{n}\left(F_i(\bx^{0}_{i},\bc^{0}_{i},\bw^{0}_{i})-F_i(\bx^T_{i},\bc^T_{i},\bw^{T}_{i})\right)}{n}$.

\textbf{Choice of $\eta_3$.} Assuming $\tau \leq \sqrt{T}$ we can take $\eta_3 = \frac{1}{4\lambda_p\sqrt{T}}$, details of this choice is discussed in the end of this section, and after some algebra we have the end result:
\begin{align*} 
	\frac{1}{T}\sum_{t=0}^{T-1}\frac{1}{n}\sum_{i=1}^{n} \|\bG^{t}_{i}\|^2 & \leq   \frac{54L_{\max}^2\tau\kappa(1+G_{Q_1}^2+G^2_{Q_2})+54L_{\max}^2+576L_{\max}^2\lambda_p \Delta_F}{\sqrt{T}} \\
	& \hspace{1cm}+ \frac{1512L_{\max}^2\tau^2\kappa+\frac{3}{16}\tau^2\kappa^2((1+G_{Q_1}^2)+G^2_{Q_2})}{T} \\
	& \hspace{1cm} + \frac{6048L_{\max}^2\tau^2\kappa}{T^{\frac{3}{2}}}  + 216L_{\max}^2\kappa
\end{align*}
This concludes the proof.

\subsection{Proof of Lemma~\ref{qupel:thm2:lemma1} and Corollary~\ref{qupel:thm2:corollary diversity}}

Let us restate and prove Lemma~\ref{qupel:thm2:lemma1},
\begin{lemma*}[Restating  Lemma~\ref{qupel:thm2:lemma1}]
	\begin{align} \label{qupel:app:lemma1}
		\frac{1}{T}\sum_{t=0}^{T-1}\frac{1}{n}\sum_{i=1}^{n} \|\bw^{t}-\bw^{t}_{i}\|^2 \leq 6 \tau^2\eta_3^2\kappa 
	\end{align}
\end{lemma*}
\begin{proof}
	Let $t_c$ be the latest synchronization time before t. Define $\gamma_t = \frac{1}{n} \sum_{i=1}^{n}\|\bw^{t} - \bw^{t}_{i}\|^2$. Then:
	\begin{align*}
		\gamma_t &= \frac{1}{n} \sum_{i=1}^{n} \Big\|\bw^{tc}-\frac{\eta_3}{n} \sum_{j=t_c}^{t} \sum_{k=1}^{n} \nabla_{\bw^{j}_{k}} F_k(\bx^{j+1}_{k},\bc^{j+1}_{k},\bw^{j}_{k}-(\bw^{tc}-\eta_3 \sum_{j=t_c}^{t} \nabla_{\bw^{j}_{i}} F_i(\bx^{j+1}_{i},\bc^{j+1}_{i},\bw^{j}_{i})\Big\|^2 \\ 
		&\stackrel{\text{(a)}}{\leq} \tau  \sum_{j=t_c}^t \frac{\eta_3^2}{n} \sum_{i=1}^n \Big\|\frac{1}{n} \sum_{k=1}^{n} \nabla_{\bw^{j}_{k}} F_k(\bx^{j+1}_{k},\bc^{j+1}_{k},\bw^{j}_{k}- \nabla_{\bw^{j}_{i}} F_i(\bx^{j+1}_{i},\bc^{j+1}_{i},\bw^{j}_{i}\Big\|^2 \tag{$\star1$} \label{qupel:app:lm1star1}\\
		&= \tau  \sum_{j=t_c}^t \frac{\eta_3^2}{n} \sum_{i=1}^n \Big[  \Big\|\frac{1}{n} \sum_{k=1}^{n} \left(\nabla_{\bw^{j}_{k}} F_k(\bx^{j+1}_{k},\bc^{j+1}_{k},\bw^{j}_{k})-\nabla_{\bw^{j}} F_k(\bx^{j+1}_{k},\bc^{j+1}_{k},\bw^{j})  \right.\\
		& \hspace{2cm} \left. + \nabla_{\bw^{j}} F_k(\bx^{j+1}_{k},\bc^{j+1}_{k},\bw^{j}) \right) -\nabla_{\bw^{j}} F_i(\bx^{j+1}_{k},\bc^{j+1}_{k},\bw^{j}) \\ 
		&\hspace{2cm} +\nabla_{\bw^{j}} F_i(\bx^{j+1}_{k},\bc^{j+1}_{k},\bw^{j})- \nabla_{\bw^{j}_{i}} F_i(\bx^{j+1}_{k},\bc^{j+1}_{k},\bw^{j}_{i}\Big\|^2 \Big] \\ 
		& \leq \tau  \sum_{j=t_c}^{t_c+\tau} 3\frac{\eta_3^2}{n}  \sum_{i=1}^n \Big[\Big\|\frac{1}{n} \sum_{k=1}^{n} \left( \nabla_{\bw^{j}_{k}} F_k(\bx^{j+1}_{k},\bc^{j+1}_{k},\bw^{j}_{k})-\nabla_{\bw^{j}} F_k(\bx^{j+1}_{k},\bc^{j+1}_{k},\bw^{j})\right)\Big\|^2\\ 
		&\hspace{2cm} + \Big\|\frac{1}{n}\sum_{k=1}^{n} \nabla_{\bw^{j}} F_k(\bx^{j+1}_{k},\bc^{j+1}_{k},\bw^{j}) -\nabla_{\bw^{j}} F_i(\bx^{j+1}_{i},\bc^{j+1}_{i},\bw^{j})\Big\|^2 \\ 
		&\hspace{3cm} + \Big\|\nabla_{\bw^{j}} F_i(\bx^{j+1}_{i},\bc^{j+1}_{i},\bw^{j})- \nabla_{\bw^{j}_{i}} F_i(\bx^{j+1}_{i},\bc^{j+1}_{i},\bw^{j}_{i}\Big\|^2\Big] \\ 
		& \leq \tau  \sum_{j=t_c}^{t_c+\tau} 3\frac{\eta_3^2}{n}  \sum_{i=1}^n \Big[\frac{4\lambda_p^2 n}{n^2}\sum_{k=1}^n\| \bw^{j}_{k}-\bw^{j}\|^2 + \kappa_i + 4\lambda_p^2\|\bw^j-\bw^{j}_{i}\|^2\Big] \\ &=
		\tau  \sum_{j=t_c}^{t_c+\tau} 3\eta_3^2(4\lambda_p^2\gamma_j+\kappa+4\lambda_p^2 \gamma_j) \tag{$\star2$} \label{qupel:app:lm1star2}
	\end{align*}
	in (a) we use the facts that  $\|\sum_{i=1}^K a_i\|^2 \leq K \sum_{i=1}^K \|a_i\|^2$, $t\leq \tau + t_c$ and that we are summing over non-negative terms. As a result, we have:
	\begin{align*}
		\gamma_t &\leq \tau  \sum_{j=t_c}^{t_c+\tau} 3\eta_3^2(8\lambda_p^2\gamma_j+\kappa)\\
		\Longrightarrow \sum_{t=t_c}^{t_c+\tau} \gamma_t &\leq \sum_{t=t_c}^{t_c+\tau}  \sum_{j=t_c}^{t_c+\tau} 3\tau\eta_3^2(8\lambda_p^2\gamma_j+\kappa) = 24\tau^2\eta_3^2\lambda_p^2 \sum_{j=t_c}^{t_c+\tau} \gamma_j + 3\tau^3 \eta_3^2\kappa
	\end{align*}
	Let us choose $\eta_3$ such that $24\tau^2\eta_3^2\lambda_p^2 \leq \frac{1}{2} \Leftrightarrow \eta_3 \leq \sqrt{\frac{1}{48\tau^2\lambda_p^2}} $, sum over all syncronization times, and divide both sides by $T$:
	\begin{align*} 
		&\frac{1}{T} \sum_{t=0}^{T-1} \gamma_t \leq \frac{1}{2} \sum_{j=0}^{T-1} \gamma_j + 3\tau^2 \eta_3^2\kappa \\ \Longrightarrow &\frac{1}{T} \sum_{t=0}^{T-1} \gamma_t \leq  6\tau^2\eta_3^2\kappa
	\end{align*}
\end{proof}
Let us restate and prove Corollary~\ref{qupel:thm2:corollary diversity}.
\begin{corollary*}[Restating Corollary~\ref{qupel:thm2:corollary diversity}]
	Recall, $\bg^{t} = \frac{1}{n} \sum_{i=1}^n \nabla_{\bw^{t}} F_i(\bx^{t+1}_{i},\bc^{t+1}_{i},\bw^{t}_{i})$. Then, we have:
	\begin{align*}
		\frac{1}{T}\sum_{t=0}^{T-1} \frac{1}{n} \sum_{i=1}^n \Big\|\bg^{t} - \nabla_{\bw^{t}_{i}} F_i(\bx^{t+1}_{i},\bc^{t+1}_{i},\bw^{t}_{i})\Big\|^2 \leq 36\lambda_p^2\tau^2\eta_3^2\kappa+3\kappa
	\end{align*}
\end{corollary*}
\begin{proof}
	
	From \eqref{qupel:app:lm1star1} $\leq$ Lemma~\ref{qupel:app:lm1star2} in the proof of \eqref{qupel:thm2:lemma1}, we have:
	
	\begin{align*}
		\sum_{t=t_c}^{t_c+\tau} \frac{1}{n} \sum_{i=1}^n \Big\|\bg^{t} - \nabla_{\bw^{t}_{i}} F_i(\bx^{t+1}_{i},\bc^{t+1}_{i},\bw^{t}_{i})\Big\|^2 \leq \sum_{j=t_c}^{t_c+\tau} 3(8\lambda_p^2\gamma_j+\kappa)
	\end{align*}
	
	Summing over all $t_c$ and dividing by $T$:
	
	\begin{align*}
		\frac{1}{T}\sum_{t=0}^{T-1} \frac{1}{n} \sum_{i=1}^n \Big\|\bg^{t} - \nabla_{\bw^{t}_{i}} F_i(\bx^{t+1}_{i},\bc^{t+1}_{i},\bw^{t}_{i})\Big\|^2 & \leq 24\lambda_p^2 \frac{1}{T} \sum_{t=0}^{T-1} \gamma_t + 3\kappa\\
		& \stackrel{\text{(a)}}{\leq} 144\lambda_p^2 \tau^2 \eta_3^2 \kappa + 3 \kappa
	\end{align*}
	where (a) is from \eqref{qupel:thm2:lemma1}.
	
	\subsection{Choice of $\eta_3$}
	
	Note that, in Lemma~\ref{qupel:thm2:lemma1} we chose $\eta_3$ such that $\eta_3 \leq \frac{1}{\sqrt{48}\lambda_p\tau}$. Now, we further introduce upper bounds on $\eta_3$. 
	\begin{itemize}
		\item We can choose $\eta_3$ small enough so that $L_{\min}=\eta_3-4\lambda_p\eta_3^2$; see \eqref{qupel_L_min-defn} for the definition of $L_{\min}$.
		\item We can choose $\eta_3$ small enough so that $\eta_3-4\lambda_p\eta_3^2 \geq \frac{\eta_3}{2}$. This is equivalent to choosing $ \eta_3 \leq \frac{1}{8\lambda_p}$.
	\end{itemize}
	
	These two choices implies $L_{\min} \geq \frac{\eta_3}{2}$. 
	
	In the end, we have 2 critical constraints on $\eta_3, \{\eta_3:\eta_3 \leq \frac{1}{\sqrt{48}\lambda_p\tau},\eta_3 \leq \frac{1}{8\lambda_p}\} $ . Then, let $\{\eta_3:\eta_3 \leq \frac{1}{8\lambda_p\tau}\}$. Moreover, assuming $\tau \leq \sqrt{T}$ we can take $\eta_3 = \frac{1}{8\lambda_p\sqrt{T}} $ this choice clearly satisfies the above constraints.
	
	From \eqref{qupel:thm2:res1} we have,
	\begin{align*} 
		\nonumber \frac{1}{T}\sum_{t=0}^{T-1}\frac{1}{n}\sum_{i=1}^{n} \Big\|\bG^{t}_{i}\Big\|^2 & \leq  36\frac{L_{\max}^2}{L_{\min}} \Big[6\tau^2\eta_3^2\kappa(\lambda_p(1+G^2_{Q_1}+G^2_{Q_2})+28\eta_3\lambda_p^2+112\eta_3^2\lambda_p^3) \notag \\
		& \hspace{1cm}+3\eta_3\kappa+12\lambda_p\eta_3^2\kappa+ \frac{\Delta_F}{T}\Big] + 12\lambda_p^2((1+G_{Q_1})^2+G^2_{Q_2})\tau^2\eta_3^2\kappa\\
		& \leq  72\frac{L_{\max}^2}{\eta_3} \Big[6\tau^2\eta_3^2\kappa(\lambda_p(1+G^2_{Q_1}+G^2_{Q_2})+28\eta_3\lambda_p^2+112\eta_3^2\lambda_p^3) \notag \\
		& \hspace{1cm}+3\eta_3\kappa+12\lambda_p\eta_3^2\kappa+ \frac{\Delta_F}{T}\Big] + 12\lambda_p^2((1+G_{Q_1})^2+G^2_{Q_2})\tau^2\eta_3^2\kappa \\
		& =  72L_{\max}^2 \Big[6\tau^2\eta_3\kappa(\lambda_p(1+G^2_{Q_1}+G^2_{Q_2})+28\eta_3\lambda_p^2+112\eta_3^2\lambda_p^3) \notag \\
		& \hspace{1cm}+3\kappa+12\lambda_p\eta_3\kappa+ \frac{\Delta_F}{\eta_3T}\Big] + 12\lambda_p^2((1+G_{Q_1})^2+G^2_{Q_2})\tau^2\eta_3^2\kappa \\
		\text{Now, we plug in $\eta_3 = \frac{1}{8\lambda_p\sqrt{T}}$:} \\
		& = 72L_{\max}^2 \Big[ \frac{3}{4}\tau^2\kappa\frac{(1+G_{Q_1}^2+G^2_{Q_2})}{\sqrt{T}}+21
		\tau^2\kappa\frac{1}{T} + 84\tau^2\kappa\frac{1}{T^{\frac{3}{2}}}\\
		& \hspace{1cm }+3\kappa + \frac{3}{4}\frac{1}{\sqrt{T}}+\frac{8\lambda_p\Delta_F}{\sqrt{T}}\Big]+\frac{3}{16}((1+G_{Q_1}^2)+G^2_{Q_2})\tau^2\kappa^2\frac{1}{T}\\
		& =  \frac{54L_{\max}^2\tau\kappa(1+G_{Q_1}^2+G^2_{Q_2})+54L_{\max}^2+576L_{\max}^2\lambda_p \Delta_F}{\sqrt{T}} \\
		& \hspace{1cm}+ \frac{1512L_{\max}^2\tau^2\kappa+\frac{3}{16}\tau^2\kappa^2((1+G_{Q_1}^2)+G^2_{Q_2})}{T} \\
		& \hspace{1cm} + \frac{6048L_{\max}^2\tau^2\kappa}{T^{\frac{3}{2}}}  + 216L_{\max}^2\kappa
	\end{align*}
	where $L_{\max}$ is defined in \eqref{qupel_L_max-defn}.
	
	This completes the proof of Theorem~\ref{qupel:thm:personalized}.
\end{proof}
